# Supplementary material for: Structural Adversarial Objectives for Self-Supervised Representation Learning
Source: arXiv:2310.00357 source file (2023-10-04)
Supplement: Supplementary file 1 [file supp_table.tex]

\begin{table*}[h]
   \centering
   \setlength{\tabcolsep}{9pt}
   \begin{tabular}{@{}c|c|c|c|c|c|c}
      \toprule
      \multirow{2}{*}{Method / Loss} &
         \multicolumn{2}{c|}{Parameters (M)} &
         \multirow{2}{*}{IS $\uparrow$} &
         \multirow{2}{*}{FID $\downarrow$} &
         \multirow{2}{*}{K-Means} &
         \multirow{2}{*}{SVM}\\
      & Discriminator & Generator &&&&\\
      \HLINE
      \vspace{-10pt}&&&&\\
      {\text BigGAN}~\cite{brock2018large}& 4.2 & 4.3 & 8.22 & 17.50 & 29.69 & 69.31\\
      \hline
      {\text StyleGAN2-ADA}\textsuperscript{\ref{cite:stylegan2_ada}}& 20.7 & 19.9 & \textbf{9.82} &\textbf{3.60} & 28.96 & 76.50\\
      \hline
      Hinge Loss &  11.5 & 4.9& 8.13& 18.54  & 36.41 & 77.19 \\
      \hline
      Hinge Loss + $\mathcal{L}_{\text{cluster}}$  &  11.5  & 4.9 & 8.07 &  24.57 & 17.99 & 76.50\\
      \hline
      Eq.~\ref{eqn:Gaussian} only, $D_B$ &   11.5  & 4.9 & 8.39& 17.83 & 70.76 & 87.9\\
      \hline
      Eq.~\ref{eqn:Gaussian} only, $\rm{JSD}$ &  11.5 &4.9&8.55& 16.97 & \textbf{80.55} & 88.32\\
      \hline
      Full Objectives & 11.5 &4.9 & 8.73& 13.63 & 80.11 & \textbf{89.76}\\
      \bottomrule
   \end{tabular}
\vspace{-3pt}
\caption{%
We extend the Table~\ref{tab:img quality table} by including two extra settings: (1) StyleGAN2-ADA\textsuperscript{\ref{cite:stylegan2_ada}} and (2) Hinge loss with $\mathcal{L}_{\rm{cluster}}$  (row 4), and two additional columns to compare model parameter counts.
Compared to BigGAN \cite{brock2018large}, both StyleGAN2-ADA and Hinge Loss (row 3) leverage a bigger model to improve the feature learning performance in the discriminator.  However, the 
primary boost in feature learning still results from our variants adopting structural objectives (last three rows). 
}%
\label{tab:sup table}
\end{table*}
